# Supplementary material for: A Novel Unsupervised Post-Processing Calibration Method for DNNS with Robustness to Domain Shift
Source: arXiv:1911.11195 source file (2019-11-25)
Supplement: Supplementary file 9 [file table_brier_std.tex]

\begin{table}[H]
\begin{center}
\caption{Brier Score$\downarrow$ for UTS and other post-processing approaches. The mean and std are reported in $20$ independent runs.}\label{table:brier_std}
\resizebox{\textwidth}{!}{  
\begin{tabular}{lllllll}
\hline
\textbf{Dataset} & \textbf{Model} & \textbf{Uncalibrated}               & \textbf{TS}                & \textbf{UTS}               & \textbf{VS}                & \textbf{MS}       \\ \hline
Birds            & ResNet50       & \textbf{0.0017 +/- 0.0000} & \textbf{0.0017 +/- 0.0000} & \textbf{0.0017 +/- 0.0000} & \textbf{0.0017 +/- 0.0000} & 0.0043 +/- 0.0001 \\
MNIST            & Lenet-5        & 0.0015 +/- 0.0001          & \textbf{0.0012 +/- 0.0001} & 0.0014 +/- 0.0000          & 0.0015 +/- 0.0001          & 0.0016 +/- 0.0001 \\
SVHN             & ResNet110      & 0.0066 +/- 0.0001          & \textbf{0.0061 +/- 0.0001} & 0.0062 +/- 0.0001          & 0.0065 +/- 0.0001          & 0.0066 +/- 0.0001 \\
SVHN             & DenseNet100    & 0.0066 +/- 0.0001          & 0.0065 +/- 0.0001          & 0.0065 +/- 0.0001          & \textbf{0.0063 +/- 0.0001} & 0.0064 +/- 0.0001 \\
CIFAR10          & DenseNet40     & 0.0118 +/- 0.0001          & \textbf{0.0109 +/- 0.0001} & 0.0115 +/- 0.0002          & 0.0121 +/- 0.0002          & 0.0118 +/- 0.0001 \\
CIFAR10          & DenseNet100    & 0.0080 +/- 0.0002          & \textbf{0.0075 +/- 0.0002} & 0.0076 +/- 0.0002          & 0.0084 +/- 0.0005          & 0.0080 +/- 0.0003 \\
CIFAR10          & ResNet110      & 0.0108 +/- 0.0002          & \textbf{0.0098 +/- 0.0001} & 0.0100 +/- 0.0001          & 0.0110 +/- 0.0003          & 0.0108 +/- 0.0002 \\
CIFAR10          & VGG16          & 0.0108 +/- 0.0002          & \textbf{0.0098 +/- 0.0003} & 0.0102 +/- 0.0003          & 0.0106 +/- 0.0002          & 0.0107 +/- 0.0002 \\
CIFAR100         & DenseNet40     & 0.0040 +/- 0.0000          & \textbf{0.0039 +/- 0.0000} & \textbf{0.0039 +/- 0.0000} & 0.0048 +/- 0.0001          & 0.0052 +/- 0.0002 \\
CIFAR100         & DenseNet100    & 0.0037 +/- 0.0000          & \textbf{0.0033 +/- 0.0000} & 0.0034 +/- 0.0000          & 0.0040 +/- 0.0000          & 0.0040 +/- 0.0001 \\
CIFAR100         & ResNet110      & 0.0043 +/- 0.0000          & \textbf{0.0040 +/- 0.0000} & \textbf{0.0040 +/- 0.0000} & 0.0048 +/- 0.0001          & 0.0051 +/- 0.0001 \\
CIFAR100         & WideResNet40-4 & 0.0030 +/- 0.0000          & \textbf{0.0029 +/- 0.0000} & 0.0030 +/- 0.0000          & 0.0031 +/- 0.0000          & 0.0030 +/- 0.0000 \\ \hline
\end{tabular}
}
\end{center}
\end{table}
