# Supplementary material for: A Novel Unsupervised Post-Processing Calibration Method for DNNS with Robustness to Domain Shift
Source: arXiv:1911.11195 source file (2019-11-25)
Supplement: Supplementary file 10 [file table_ece_std.tex]

\begin{table}[H]
\begin{center}
\caption{ECE$\downarrow$ for UTS and other post-processing approaches. The mean and std are reported in $20$ independent runs.}\label{table:ece_std}
\resizebox{\textwidth}{!}{  
\begin{tabular}{lllllll}
\hline
\textbf{Dataset} & \textbf{Model} & \textbf{Uncalibrated}      & \textbf{TS}                & \textbf{UTS}               & \textbf{VS}       & \textbf{MS}       \\ \hline
Birds            & ResNet50       & 0.0601 +/- 0.0015 & 0.0397 +/- 0.0025          & \textbf{0.0350 +/- 0.0024} & 0.0576 +/- 0.0019 & 0.2940 +/- 0.0089 \\
MNIST            & Lenet-5        & 0.0074 +/- 0.0004 & 0.0027 +/- 0.0009          & \textbf{0.0199 +/- 0.0014} & 0.0074 +/- 0.0004 & 0.0077 +/- 0.0005 \\
SVHN             & ResNet110      & 0.0266 +/- 0.0004 & \textbf{0.0044 +/- 0.0009} & 0.0127 +/- 0.0036          & 0.0247 +/- 0.0003 & 0.0264 +/- 0.0005 \\
SVHN             & DenseNet100    & 0.0160 +/- 0.0004 & \textbf{0.0059 +/- 0.0009} & 0.0106 +/- 0.0013          & 0.0139 +/- 0.0003 & 0.0156 +/- 0.0005 \\
CIFAR10          & DenseNet40     & 0.0409 +/- 0.0007 & \textbf{0.0070 +/- 0.0009} & 0.0351 +/- 0.0039          & 0.0410 +/- 0.0021 & 0.0419 +/- 0.0008 \\
CIFAR10          & DenseNet100    & 0.0262 +/- 0.0010 & \textbf{0.0073 +/- 0.0017} & 0.0157 +/- 0.0040          & 0.0281 +/- 0.0033 & 0.0262 +/- 0.0017 \\
CIFAR10          & ResNet110      & 0.0431 +/- 0.0009 & \textbf{0.0088 +/- 0.0009} & 0.0226 +/- 0.0021          & 0.0435 +/- 0.0023 & 0.0439 +/- 0.0012 \\
CIFAR10          & VGG16          & 0.0419 +/- 0.0010 & \textbf{0.0169 +/- 0.0009} & 0.0297 +/- 0.0043          & 0.0402 +/- 0.0011 & 0.0419 +/- 0.0011 \\
CIFAR100         & DenseNet40     & 0.0861 +/- 0.0011 & \textbf{0.0109 +/- 0.0018} & 0.0390 +/- 0.0062          & 0.1312 +/- 0.0054 & 0.1553 +/- 0.0102 \\
CIFAR100         & DenseNet100    & 0.1223 +/- 0.0016 & \textbf{0.0152 +/- 0.0011} & 0.0372 +/- 0.0063          & 0.1416 +/- 0.0020 & 0.1452 +/- 0.0039 \\
CIFAR100         & ResNet110      & 0.1265 +/- 0.0006 & \textbf{0.0102 +/- 0.0027} & 0.0447 +/- 0.0048          & 0.1567 +/- 0.0045 & 0.1740 +/- 0.0074 \\
CIFAR100         & WideResNet40-4 & 0.0894 +/- 0.0012 & \textbf{0.0402 +/- 0.0027} & 0.0689 +/- 0.0033          & 0.0839 +/- 0.0037 & 0.0850 +/- 0.0023 \\ \hline
\end{tabular}
}
\end{center}
\end{table}
